# Supplementary material for: Graph Structure Learning for Robust Graph Neural Networks
Source: arXiv:2005.10203 source file (2020-06-27)
Supplement: Supplementary file 1 [file appendix.tex]

%%
%% If your work has an appendix, this is the place to put it.

\appendix
\label{sec:appendix}
\section{Attack Methods}
We use the following code to generate adversarial attacks.
\begin{itemize}
\item Meta-attack: https://github.com/danielzuegner/gnn-meta-attack
\item Nettack: https://github.com/danielzuegner/nettack
\end{itemize}

\section{Baselines}
We use the following publicly available code of baseline methods to defend against adversarial attacks:
\begin{itemize}
\item GCN: https://github.com/tkipf/pygcn
\item GAT: https://github.com/PetarV-/GAT
\item RGCN: https://github.com/thumanlab/nrlweb/blob/master/
static/assets/download/RGCN.zip

\end{itemize}

% 
% \section{Additional Experimental Results}
% 
% \begin{figure}[htb]
% \centering
% \includegraphics[width=0.5\linewidth]{images/rank_pubmed.pdf}
% \caption{Rank growth on Pumbed under meta-attack}
% \end{figure}

% \begin{figure}[htb]
% \centering
% \includegraphics[width=0.5\linewidth]{images/pubmed_learned_adj_meta.pdf}
% \caption{Weight density distribution on learned adjacency on Pubmed dataset}
% \end{figure}
